# Supplementary material for: Error Bounds of Projection Models in Weakly Supervised 3D Human Pose Estimation
Source: arXiv:2010.12317 ancillary file (2020-10-23)
Supplement: Supplementary file 2 [file supplementary_material.pdf]

# Supplementary Material

Nikolas Klug<sup>1\*</sup> Moritz Einfalt<sup>2\*</sup> Stephan Brehm<sup>2</sup> Rainer Lienhart<sup>2</sup>

University of Augsburg

<sup>1</sup>klug.nikolas@gmail.com

<sup>2</sup>{firstname.lastname}@uni-a.de

## 1. Detailed Derivations

For the sake of completeness, we provide more detailed derivations for the best-case 3D estimates and the resulting minimal MPJPE under the normalized and weak perspective projection model.

### 1.1. Best-Case Normalized Perspective 3D Estimate

Recall that under the normalized perspective projection, the 3D pose estimate only depends on the per-point depth estimate  $\tilde{Z}_i$ . Under normalization by translation as well as scaling, the squared JPE has the same form, with

$$\begin{aligned}\Delta d_i^2(\tilde{Z}_i) &= (\tilde{Z}_i a - X_i)^2 + (\tilde{Z}_i b - Y_i)^2 + (\tilde{Z}_i - Z_i)^2 \\ &= \tilde{Z}_i^2 (a^2 + b^2 + 1) - 2\tilde{Z}_i (aX_i + bY_i - Z_i) \\ &\quad + X_i^2 + Y_i^2 + Z_i^2,\end{aligned}\quad (1)$$

where  $a$  and  $b$  are independent of  $\tilde{Z}_i$ . With  $\Delta d_i^2$  being a square function in  $\tilde{Z}_i$ , we obtain the best-case depth estimate by differentiating  $\Delta d_i^2$  w.r.t.  $\tilde{Z}_i$ :

$$\Delta d_i^{2'}(\tilde{Z}_i) = 2 \cdot (\tilde{Z}_i (a^2 + b^2 + 1) - aX_i - bY_i - Z_i). \quad (2)$$

Setting this expression equal to zero yields the optimal depth estimate  $\tilde{Z}_i^*$ , with

$$\tilde{Z}_i^* = \frac{aX_i + bY_i + Z_i}{1 + a^2 + b^2}. \quad (3)$$

#### 1.1.1 Minimal JPE under Translation Normalization

Under normalization by translation, we have  $a = \left(\frac{X_i}{Z_i} + dx\left(\frac{1}{Z_i} - \frac{1}{Z}\right)\right)$  and  $b = \frac{Y_i}{Z_i}$ . With the optimal 3D estimate  $\tilde{P}_i = (\tilde{X}_i^*, \tilde{Y}_i^*, \tilde{Z}_i^*)$ , the resulting minimal JPE for joint  $P_i$  is

$$\Delta d_i = \sqrt{(\tilde{X}_i^* - X_i)^2 + (\tilde{Y}_i^* - Y_i)^2 + (\tilde{Z}_i^* - Z_i)^2}$$

\* Authors contributed equally

$$\begin{aligned}&= \sqrt{\frac{(aY_i - bX_i)^2 + (aZ_i - X_i)^2 + (bZ_i - Y_i)^2}{1 + a^2 + b^2}} \\ &= \sqrt{\frac{dx^2 \cdot \left(\frac{1}{Z_i} - \frac{1}{Z}\right)^2 \cdot (Y_i^2 + Z_i^2)}{1 + a^2 + b^2}} \\ &= \left| dx \left( \frac{1}{Z_i} - \frac{1}{Z} \right) \right| \sqrt{\frac{Y_i^2 + Z_i^2}{1 + a^2 + b^2}}.\end{aligned}\quad (4)$$

#### 1.1.2 Minimal JPE under Scale Normalization

Under normalization by scaling, we have  $a = \rho \cdot \frac{X_i}{Z_i + dz}$  and  $b = \rho \cdot \frac{Y_i}{Z_i + dz}$ . The resulting minimal JPE for joint  $P_i$  is calculated as

$$\begin{aligned}\Delta d_i &= \sqrt{(\tilde{X}_i^* - X_i)^2 + (\tilde{Y}_i^* - Y_i)^2 + (\tilde{Z}_i^* - Z_i)^2} \\ &= \sqrt{\frac{(aY_i - bX_i)^2 + (aZ_i - X_i)^2 + (bZ_i - Y_i)^2}{1 + a^2 + b^2}} \\ &= \sqrt{\frac{\left(\rho \cdot \frac{X_i}{Z_i + dz} \cdot Z_i - X_i\right)^2 + \left(\rho \cdot \frac{Y_i}{Z_i + dz} \cdot Z_i - Y_i\right)^2}{1 + a^2 + b^2}} \\ &= \sqrt{\frac{\left(X_i^2 \left(\rho \cdot \frac{Z_i}{Z_i + dz} - 1\right)\right)^2 + \left(Y_i^2 \left(\rho \cdot \frac{Z_i}{Z_i + dz} - 1\right)\right)^2}{1 + a^2 + b^2}} \\ &= \left| 1 - \rho \cdot \frac{Z_i}{Z_i + dz} \right| \sqrt{\frac{X_i^2 + Y_i^2}{1 + a^2 + b^2}}.\end{aligned}\quad (5)$$

### 1.2. Best-Case Weak Perspective 3D Estimate

Recall that the weak perspective projection model allows a perfect depth estimate  $\tilde{Z}_i = Z_i'$ . The mean squared per-joint error for the complete pose estimate is then reduced to

$$\Delta d_2(s) = \frac{1}{n} \sum_i (X_i' - sx_i')^2 + (Y_i' - sy_i')^2$$

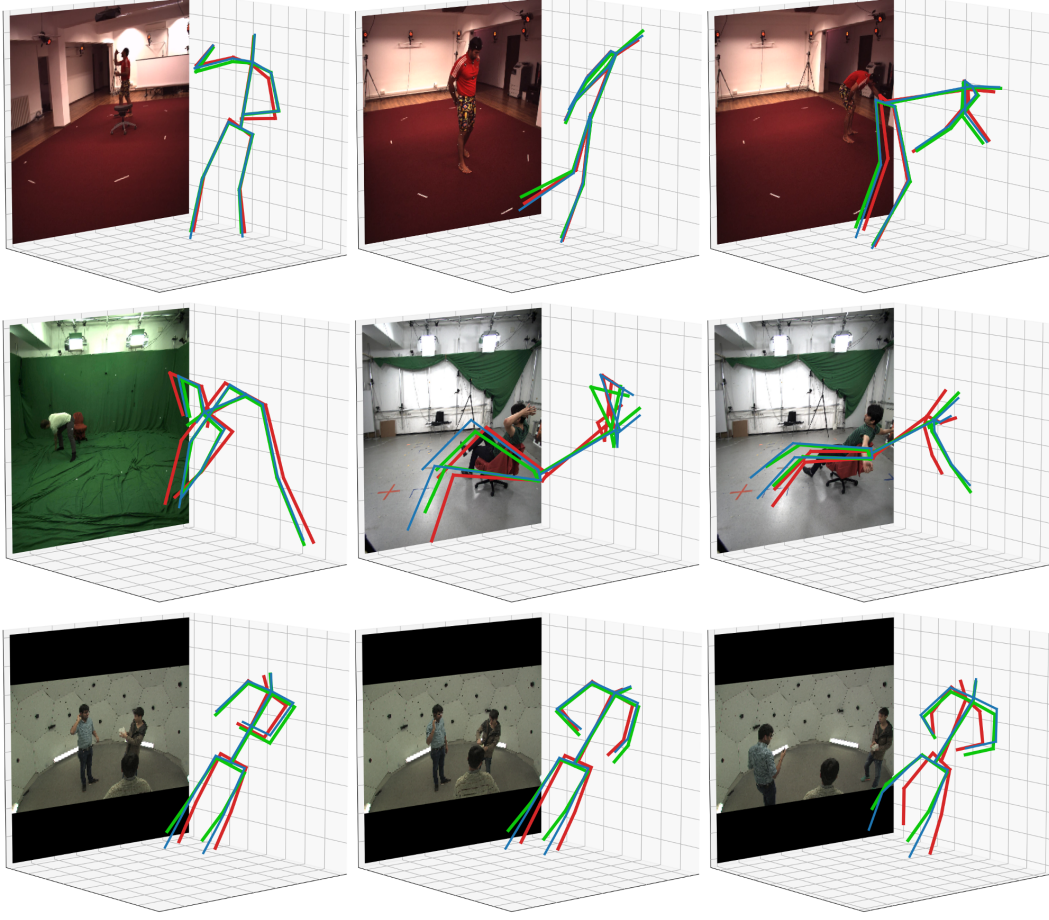

Figure 1: Top to bottom: Additional test set examples from Human3.6m, MPI-INF-3DHP and CMU Panoptic (leftmost person), respectively. The examples from left to right are selected at the 75, 90 and 99 percentiles with respect to the MPIJPE between the ground truth (red) and the best-case pose estimate under weak perspective projection (green). The best-case poses under normalized perspective projection (blue) are depicted for the same examples and follow a similar error distribution.

$$= \frac{s^2}{n} \left( \sum_i x_i'^2 + y_i'^2 \right) - \frac{2s}{n} \left( \sum_i x_i' X_i' + y_i' Y_i' \right) + \frac{1}{n} \left( \sum_i X_i'^2 + Y_i'^2 \right) b, \quad (6)$$

where  $s$  is the estimated weak perspective scaling factor for the complete pose. This is again a square function in  $s$ , with its derivative

$$\Delta d'_2(s) = \frac{2s}{n} \left( \sum_i x_i'^2 + y_i'^2 \right) - \frac{2}{n} \left( \sum_i x_i' X_i' + y_i' Y_i' \right). \quad (7)$$

Setting this expression equal to zero yields the optimal scale factor  $s^*$ , with

$$s^* = \frac{\sum_i X_i' x_i' + Y_i' y_i'}{\sum_i x_i'^2 + y_i'^2}. \quad (8)$$

## 2. Qualitative Examples

We provide additional examples of the best-case 3D human pose estimates under the normalized and weak perspective projection model. Figure 1 depicts examples from the *Human3.6m* [1], *MPI-INF-3DHP* [3] and *CMU Panoptic* [2] datasets at different MPIJPE percentiles. The inherent simplifications in the projection models lead to guaranteed and clearly visible discrepancies compared to the 3D ground truth pose. Note that the largest deviations can be observed for persons that are either clearly off-center (top right, bottom) or very close to the camera (mid), which matches our quantitative results.

## References

- [1] C. Ionescu, D. Papava, V. Olaru, and C. Sminchisescu. Human3.6M: Large Scale Datasets and Predictive Methods for 3D Human Sensing in Natural Envi-

ronments. *IEEE Transactions on Pattern Analysis and Machine Intelligence*, 36(7):1325–1339, Jul 2014. 2

- [2] H. Joo, H. Liu, L. Tan, L. Gui, B. Nabbe, I. Matthews, T. Kanade, S. Nobuhara, and Y. Sheikh. Panoptic Studio: A Massively Multiview System for Social Motion Capture. In *The IEEE International Conference on Computer Vision (ICCV)*, 2015. 2
- [3] D. Mehta, H. Rhodin, D. Casas, P. Fua, O. Sotnychenko, W. Xu, and C. Theobalt. Monocular 3D Human Pose Estimation In The Wild Using Improved CNN Supervision. *2017 International Conference on 3D Vision (3DV)*, Oct. 2017. 2
